# Supplementary material for: Sector models - A toolkit for teaching general relativity: II. Geodesics
Source: arXiv:1804.09828 ancillary file (2018-04-25)

Worksheets for

Sector models—A toolkit for teaching general relativity:

II. Geodesics

[www.spacetime.travel.org/sectormodels2](http://www.spacetime.travel.org/sectormodels2)

Arbeitsmaterialien zu

Sektormodelle – Ein Werkzeugkasten zur Vermittlung der Allgemeinen  
Relativitätstheorie: II. Geodäten

[www.tempolimit-lichtgeschwindigkeit.de/sectormodels2](http://www.tempolimit-lichtgeschwindigkeit.de/sectormodels2)

Corvin Zahn, Ute Kraus, Universität Hildesheim, 2018

Sector model of a spherical cap

Sektormodell einer Kugelkalotte

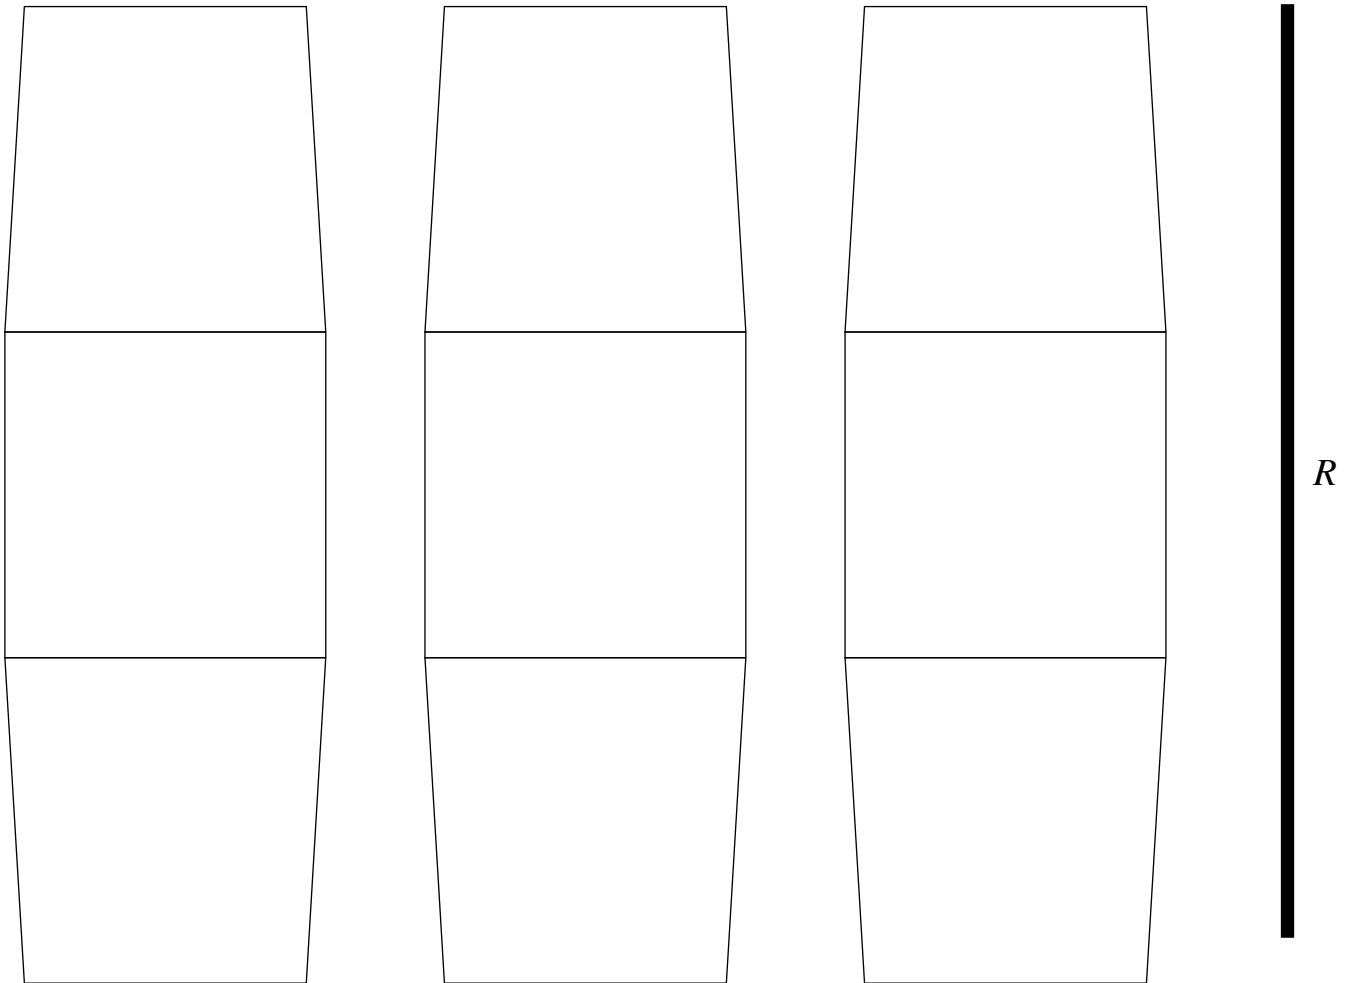

## Sector model of a spherical cap

With marking for a single geodesic

## Sektormodell einer Kugelkalotte

Mit Startstrich für eine Geodäte

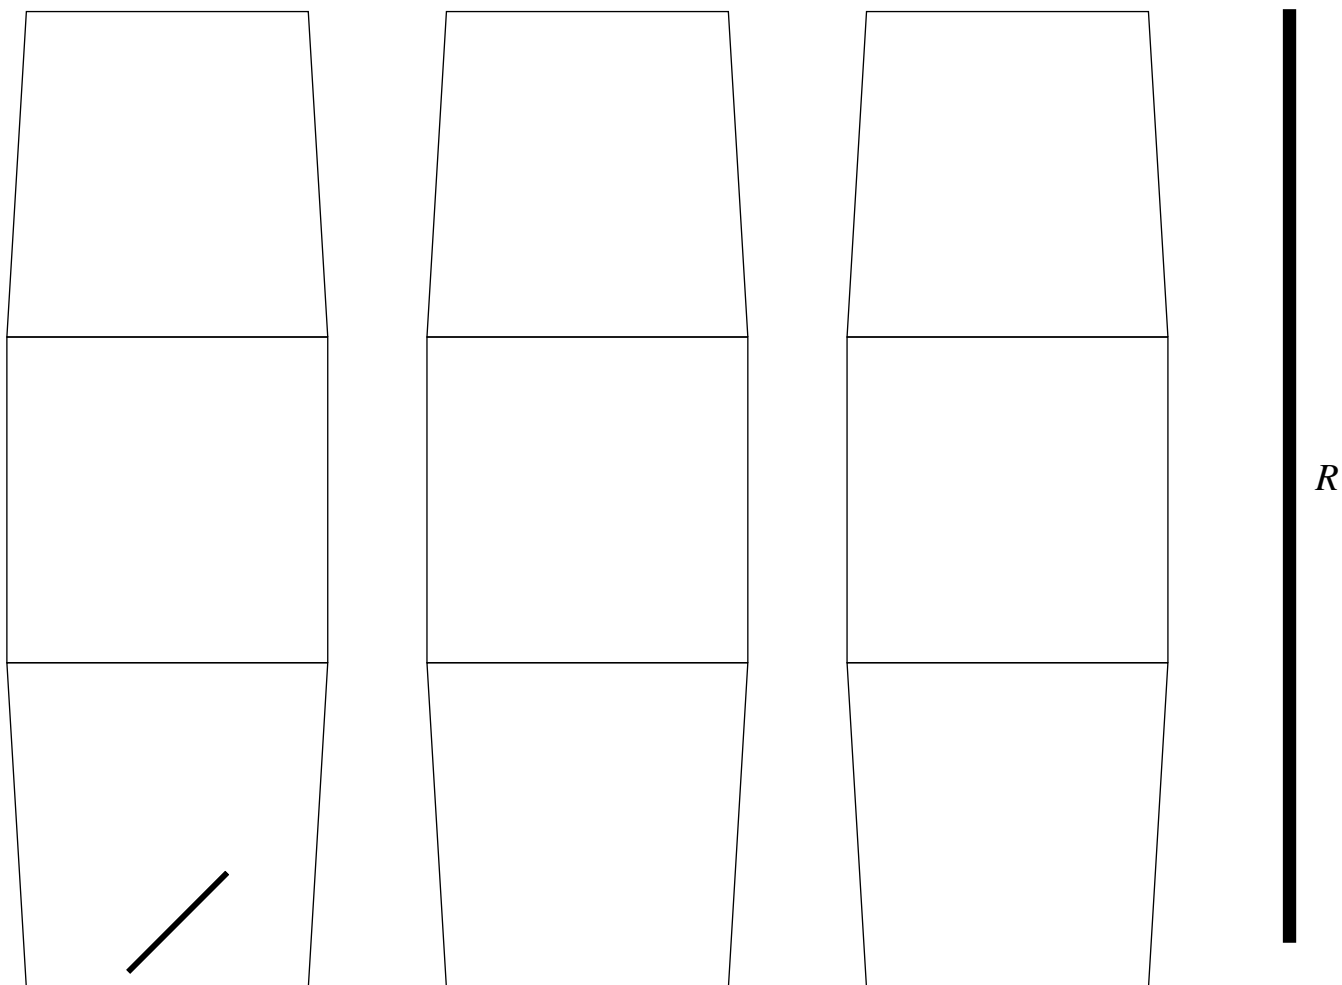

## Sector model of a spherical cap

With markings for two initially parallel geodesics

## Sektormodell einer Kugelkalotte

Mit Startstrichen für zwei parallel startende Geodäten

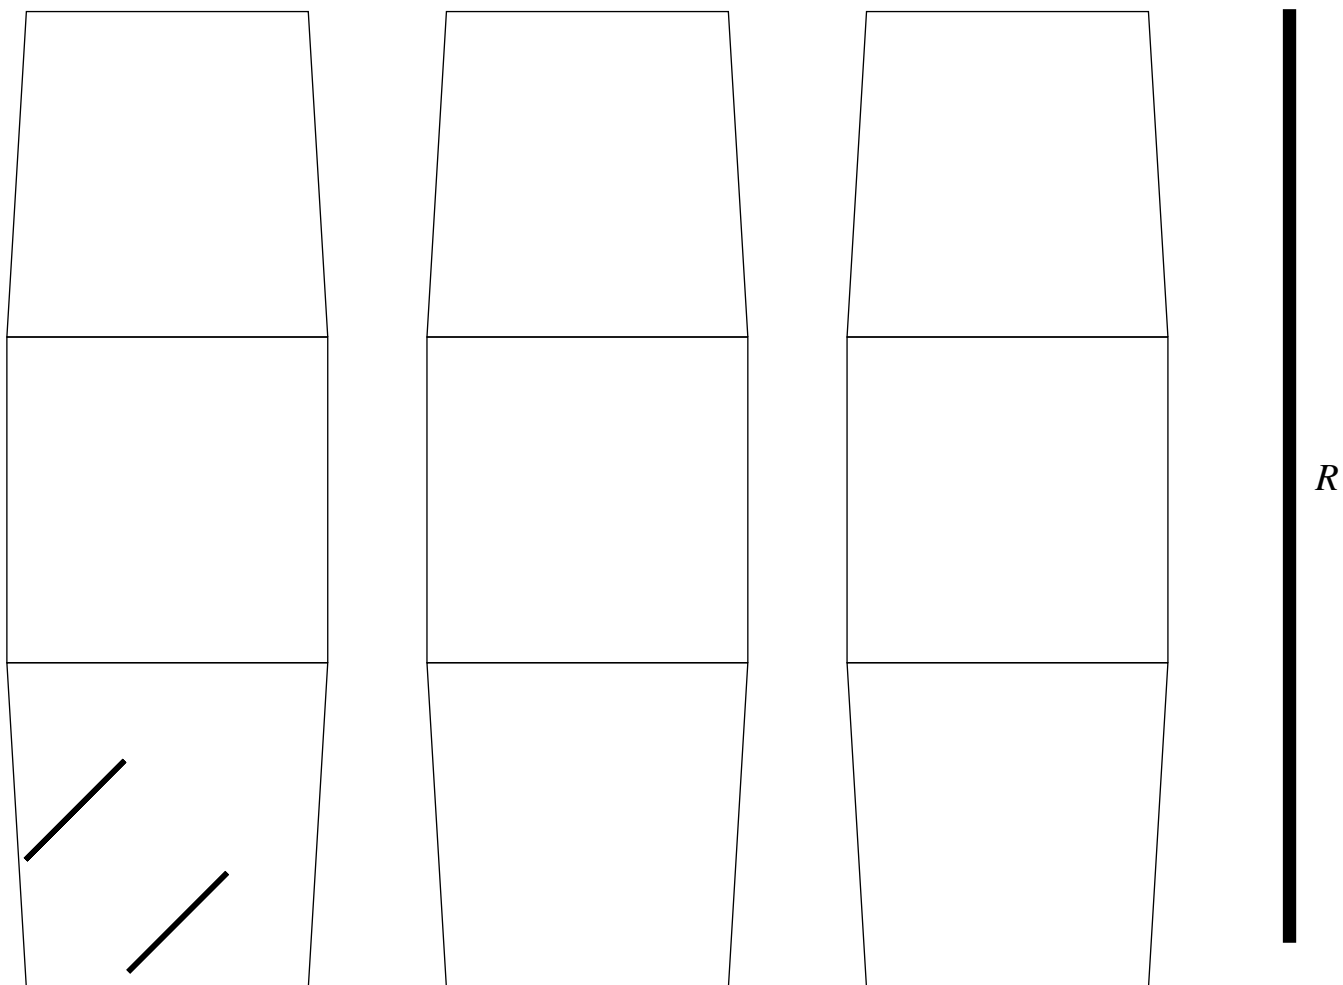

# Sector model of a spherical cap

With a single geodesic

## Sektormodell einer Kugelkalotte

Mit einer Geodäten

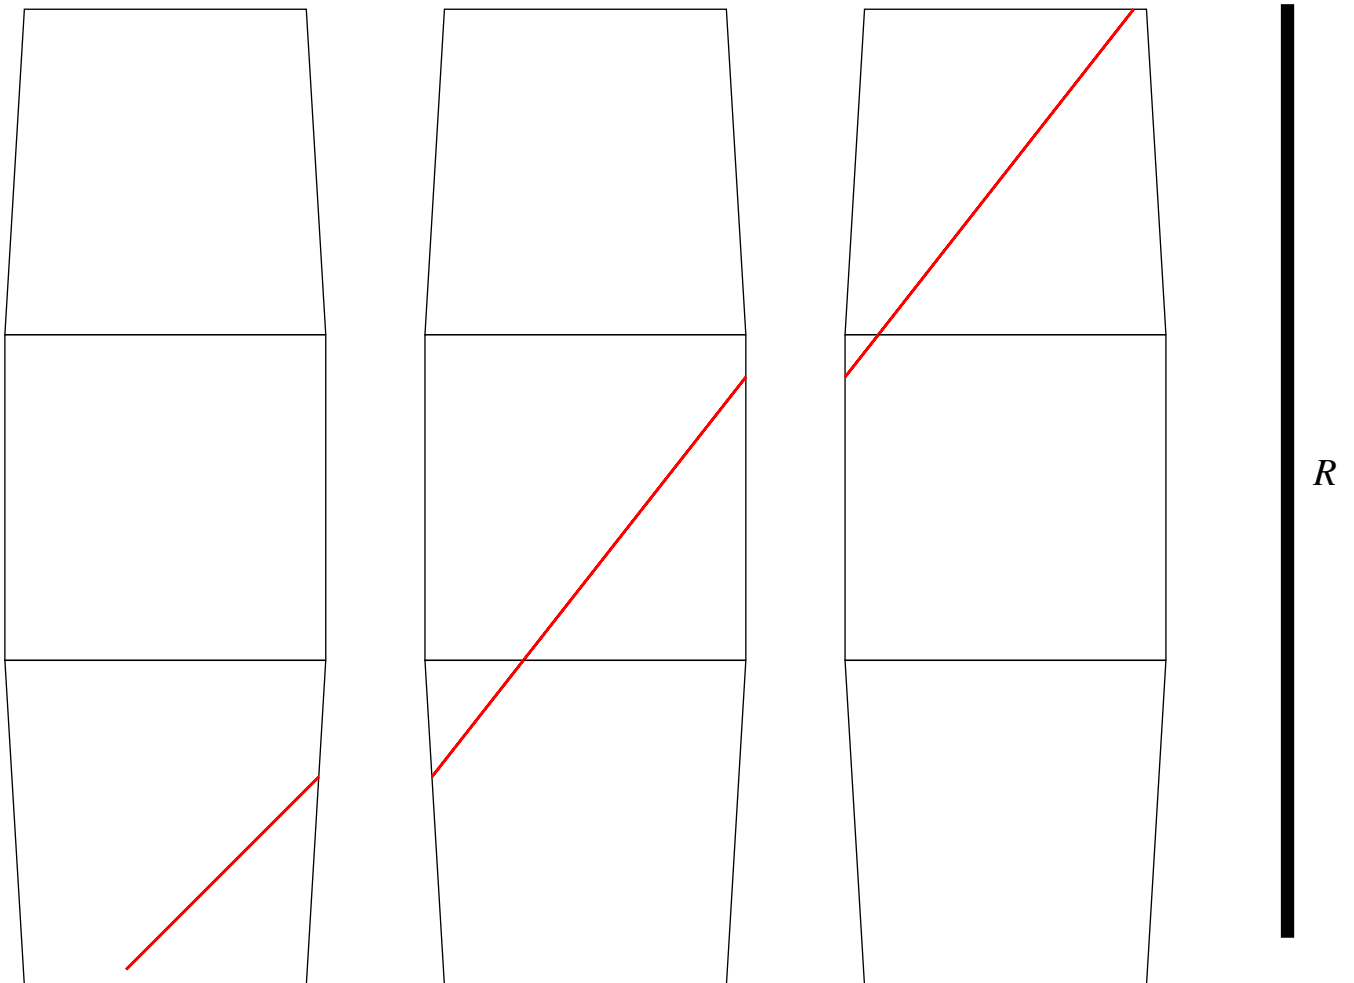

## Sector model of a spherical cap

With two initially parallel geodesics

## Sektormodell einer Kugelkalotte

Mit zwei parallel startenden Geodäten

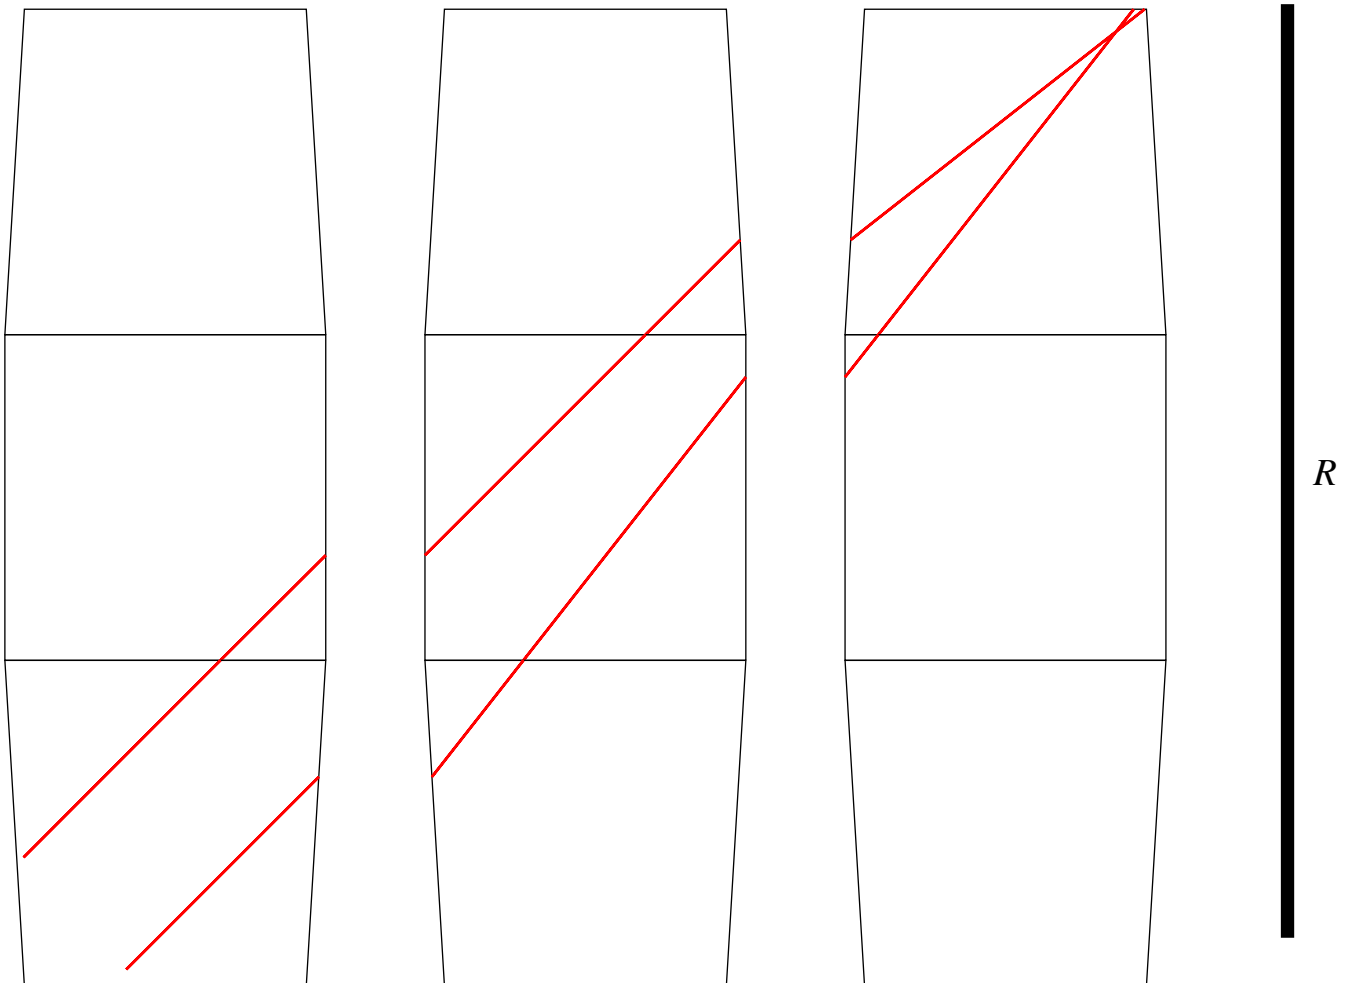

Sector model of a saddle

Sektormodell einer Sattelfläche

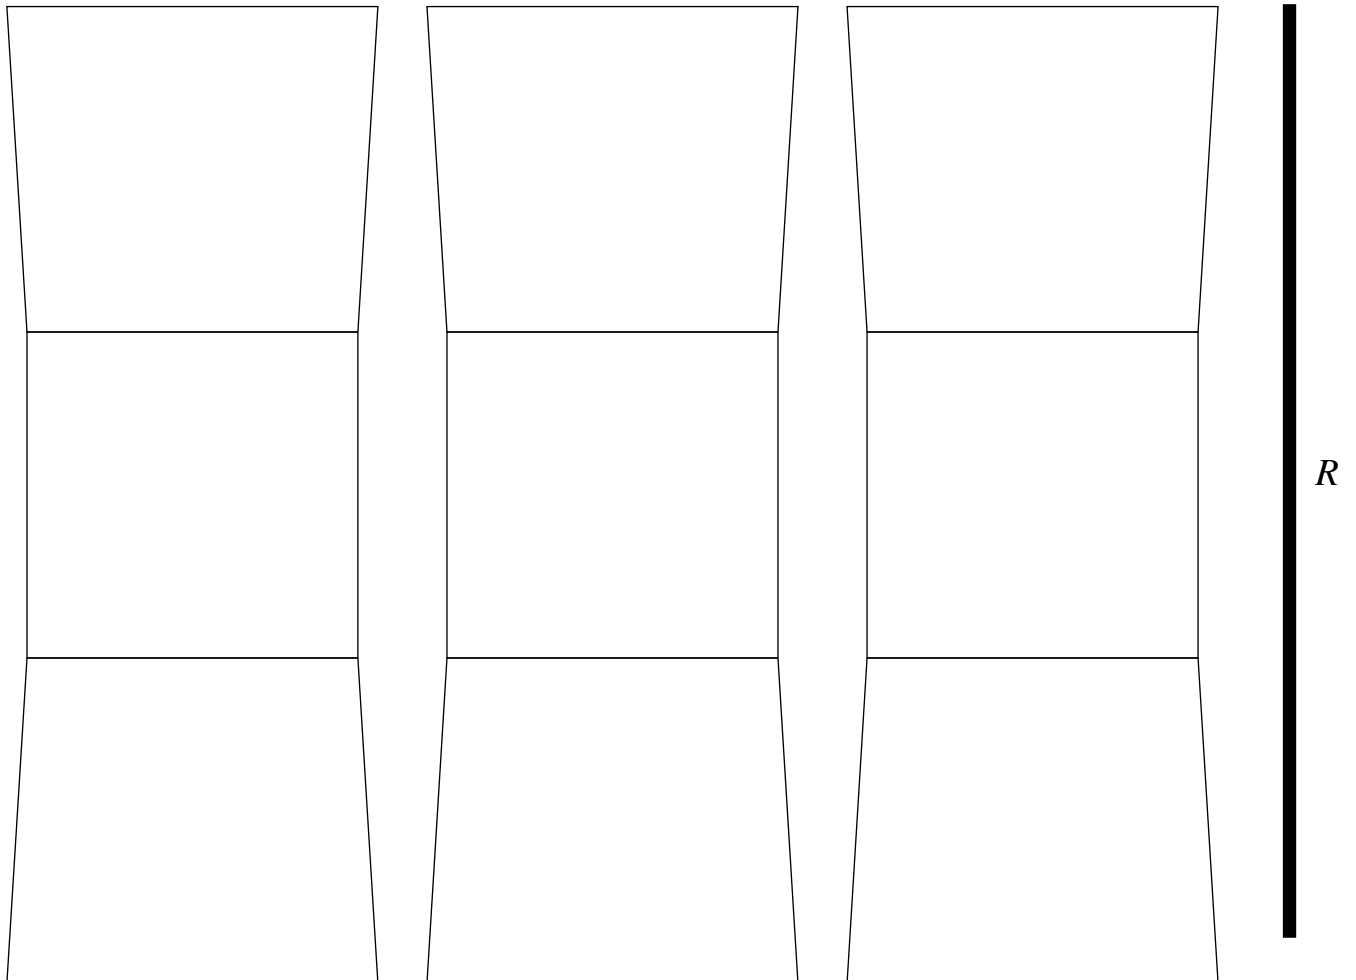

## Sector model of a saddle

With marking for a single geodesic

## Sektormodell einer Sattelfläche

Mit Startstrich für eine Geodäte

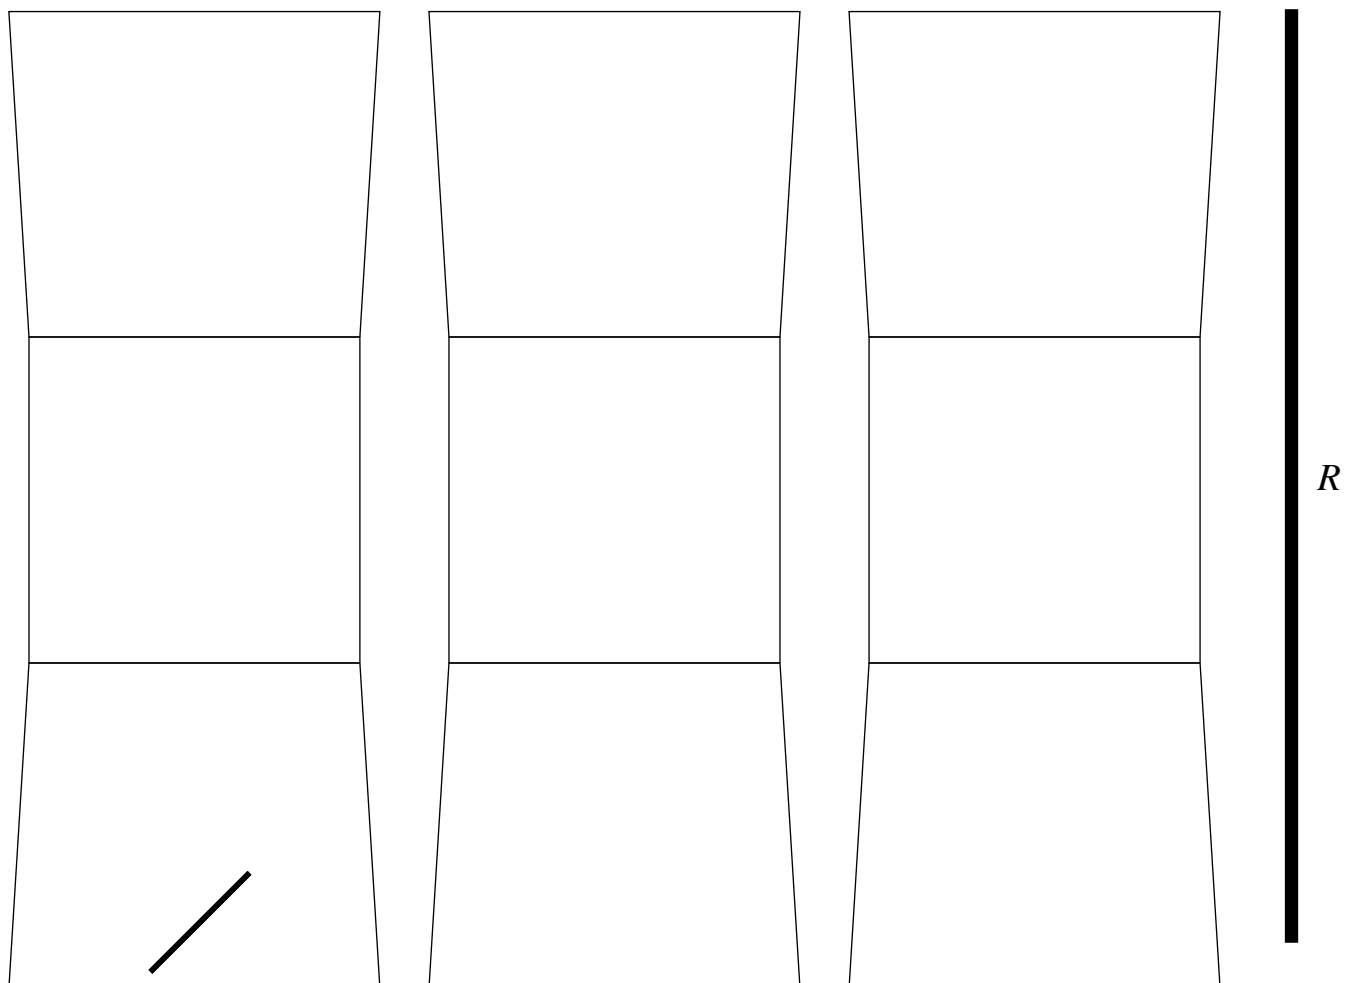



## Sector model of a saddle

With markings for two initially parallel geodesics

## Sektormodell einer Sattelfläche

Mit Startstrichen für zwei parallel startende Geodäten

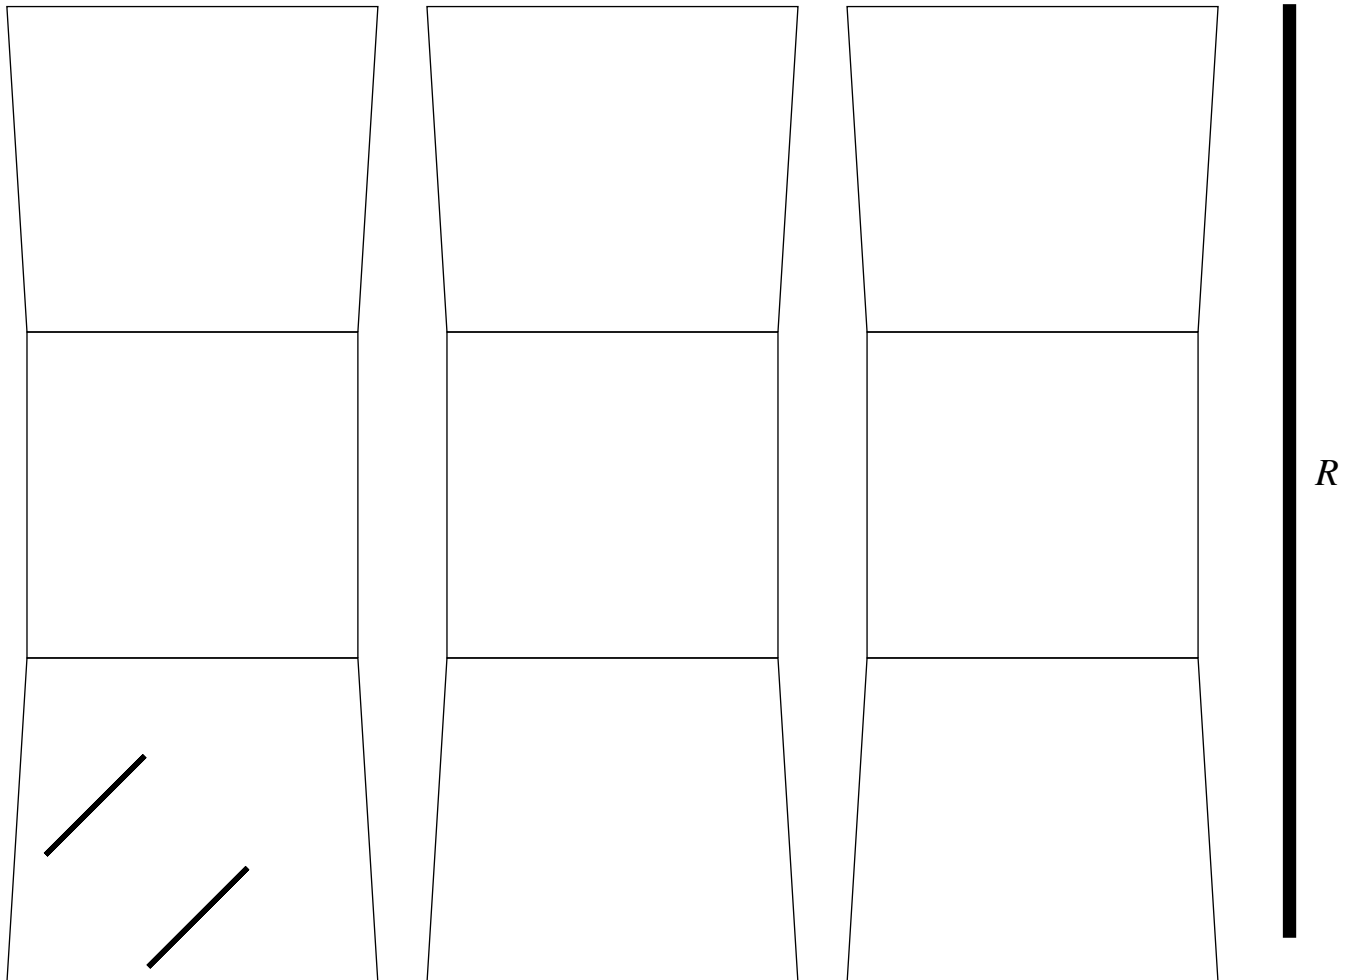

## Sector model of a saddle

With a single geodesic

## Sektormodell einer Sattelfläche

Mit einer Geodäten

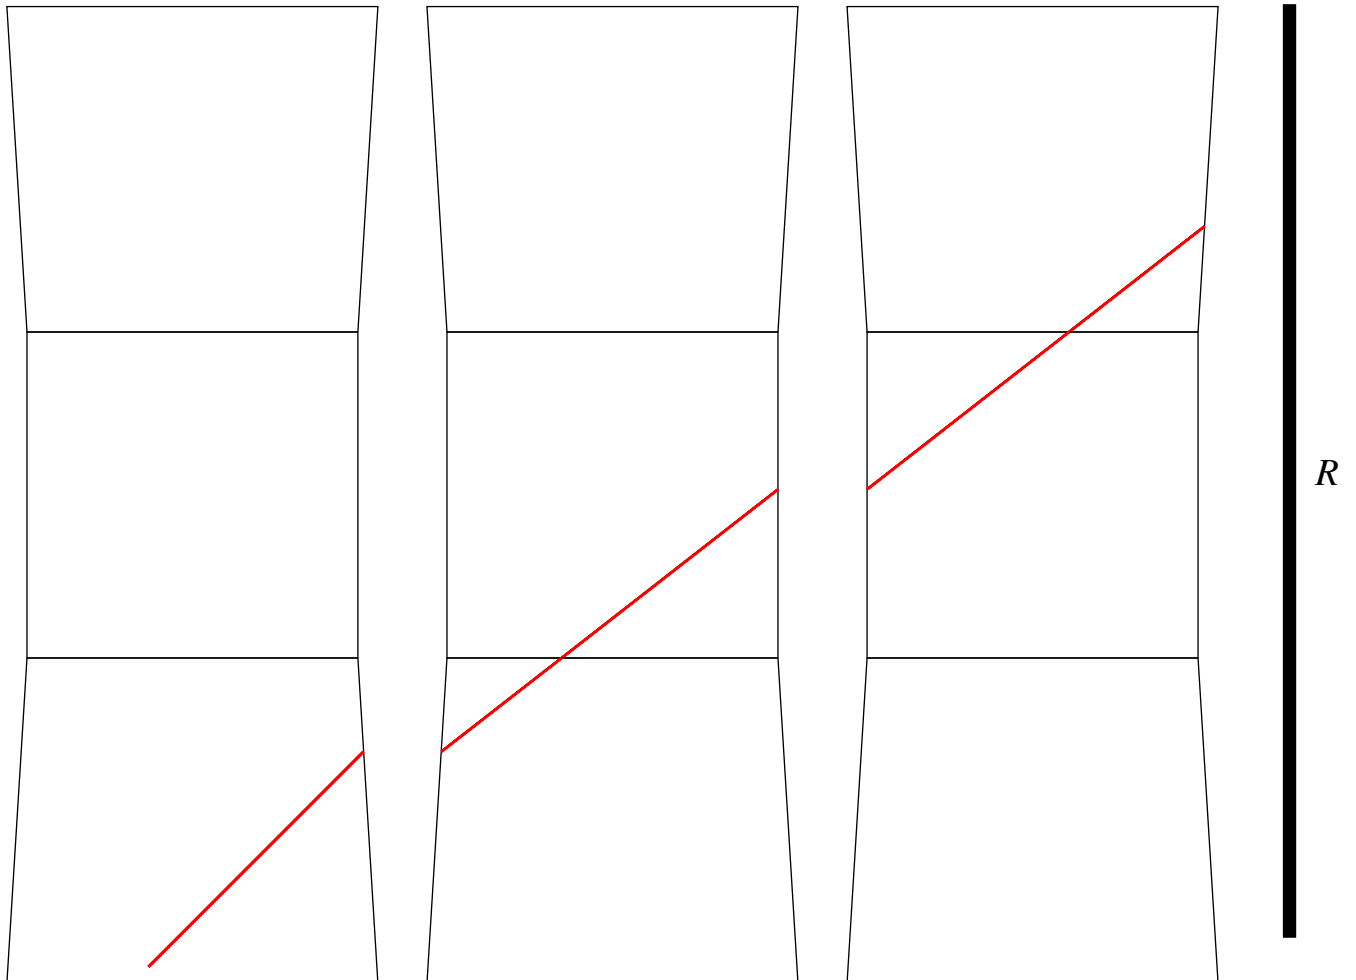

## Sector model of a saddle

With two initially parallel geodesics

## Sektormodell einer Sattelfläche

Mit zwei parallel startenden Geodäten

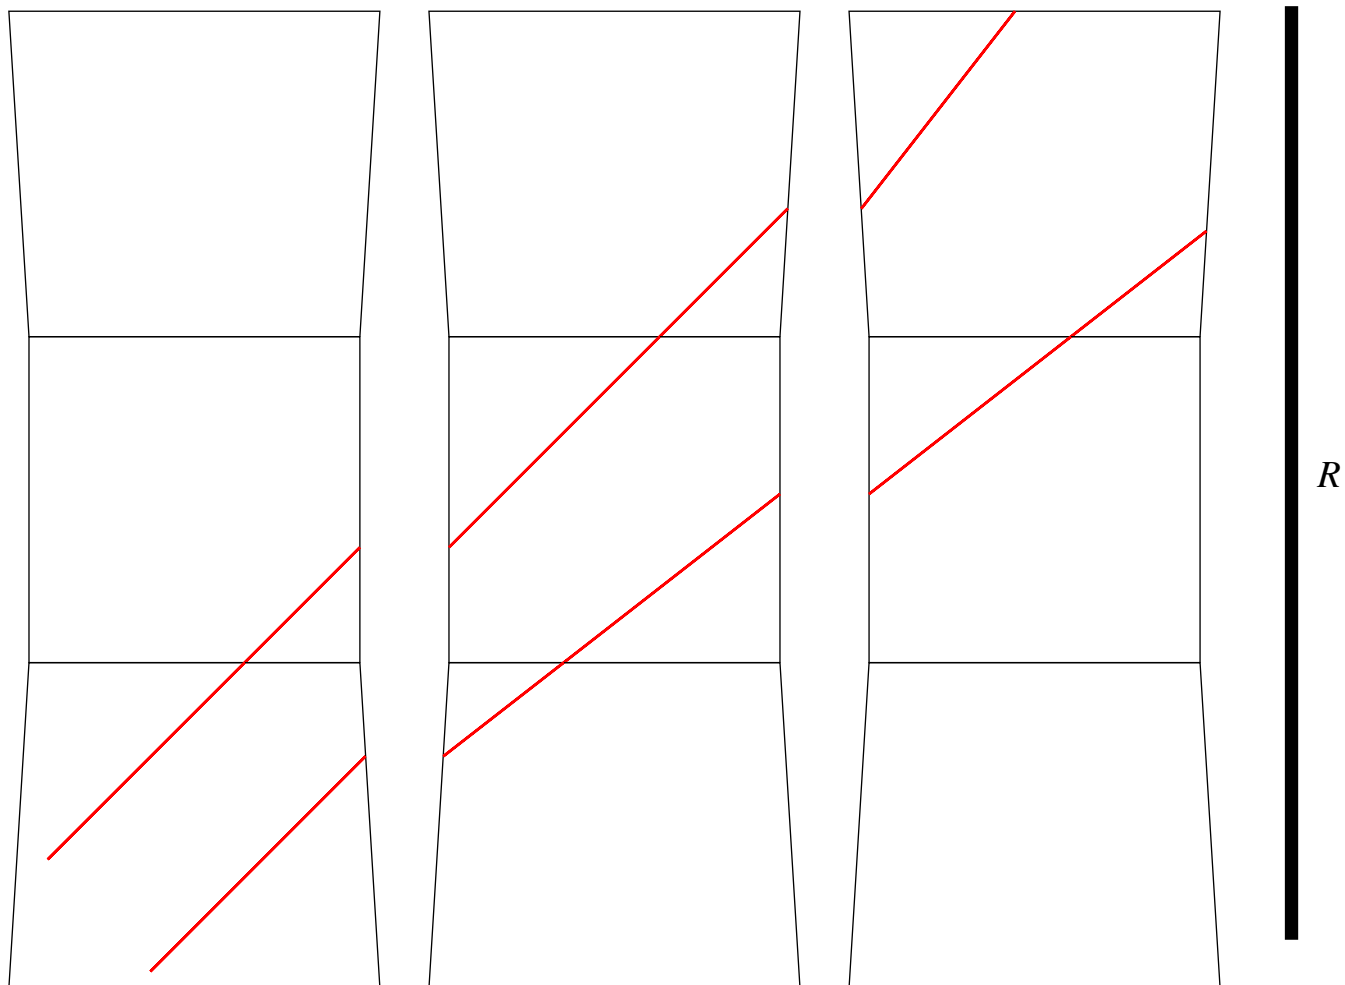

## Sector model of the equatorial plane of a black hole

Cut-out sectors for the inner and the middle ring

## Sektormodell der Äquatorfläche eines Schwarzen Lochs

Sektoren für den inneren und den mittleren Ring, zum Ausschneiden

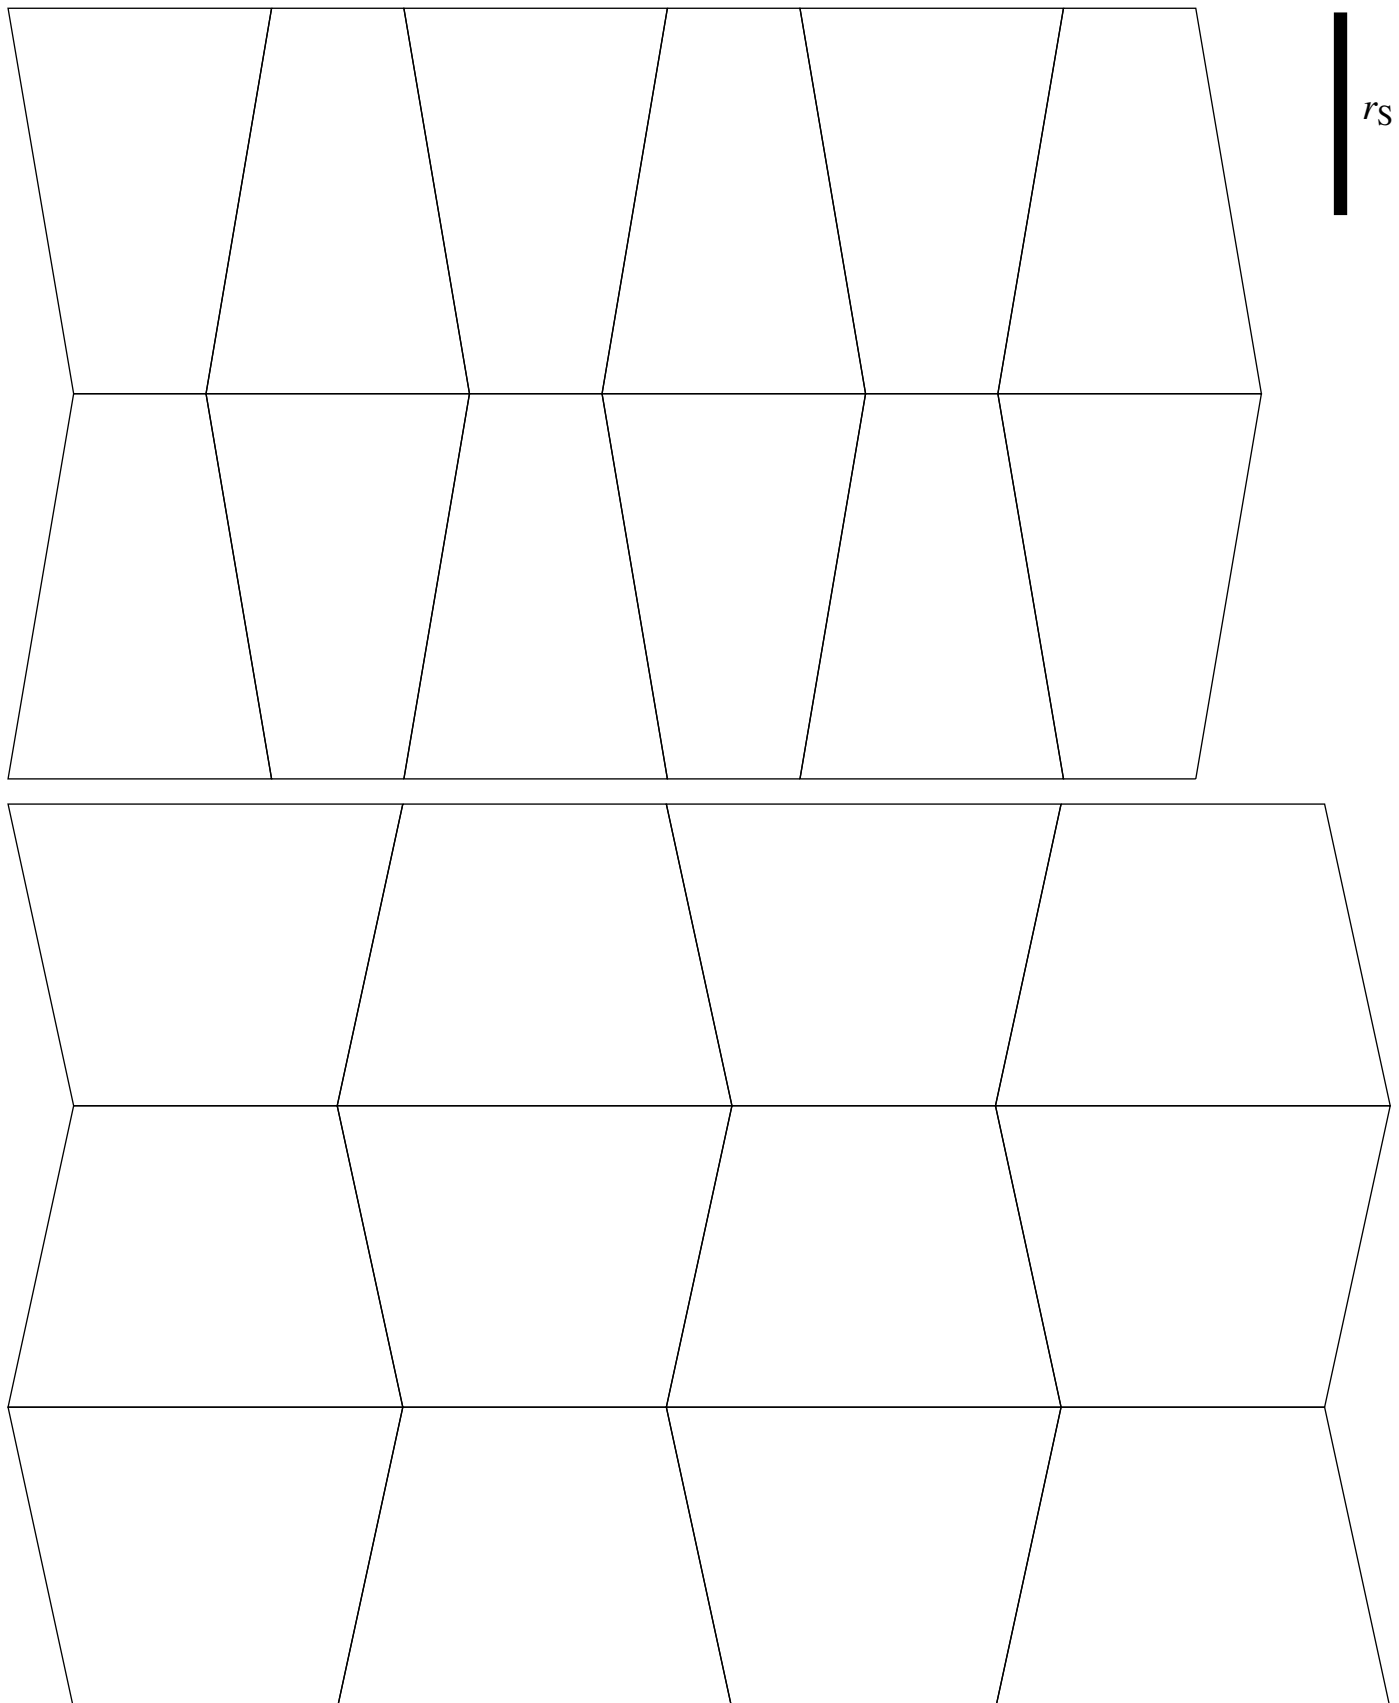

## Sector model of the equatorial plane of a black hole

Cut-out sectors for the outer ring

## Sektormodell der Äquatorfläche eines Schwarzen Lochs

Sektoren für den äußeren Ring, zum Ausschneiden

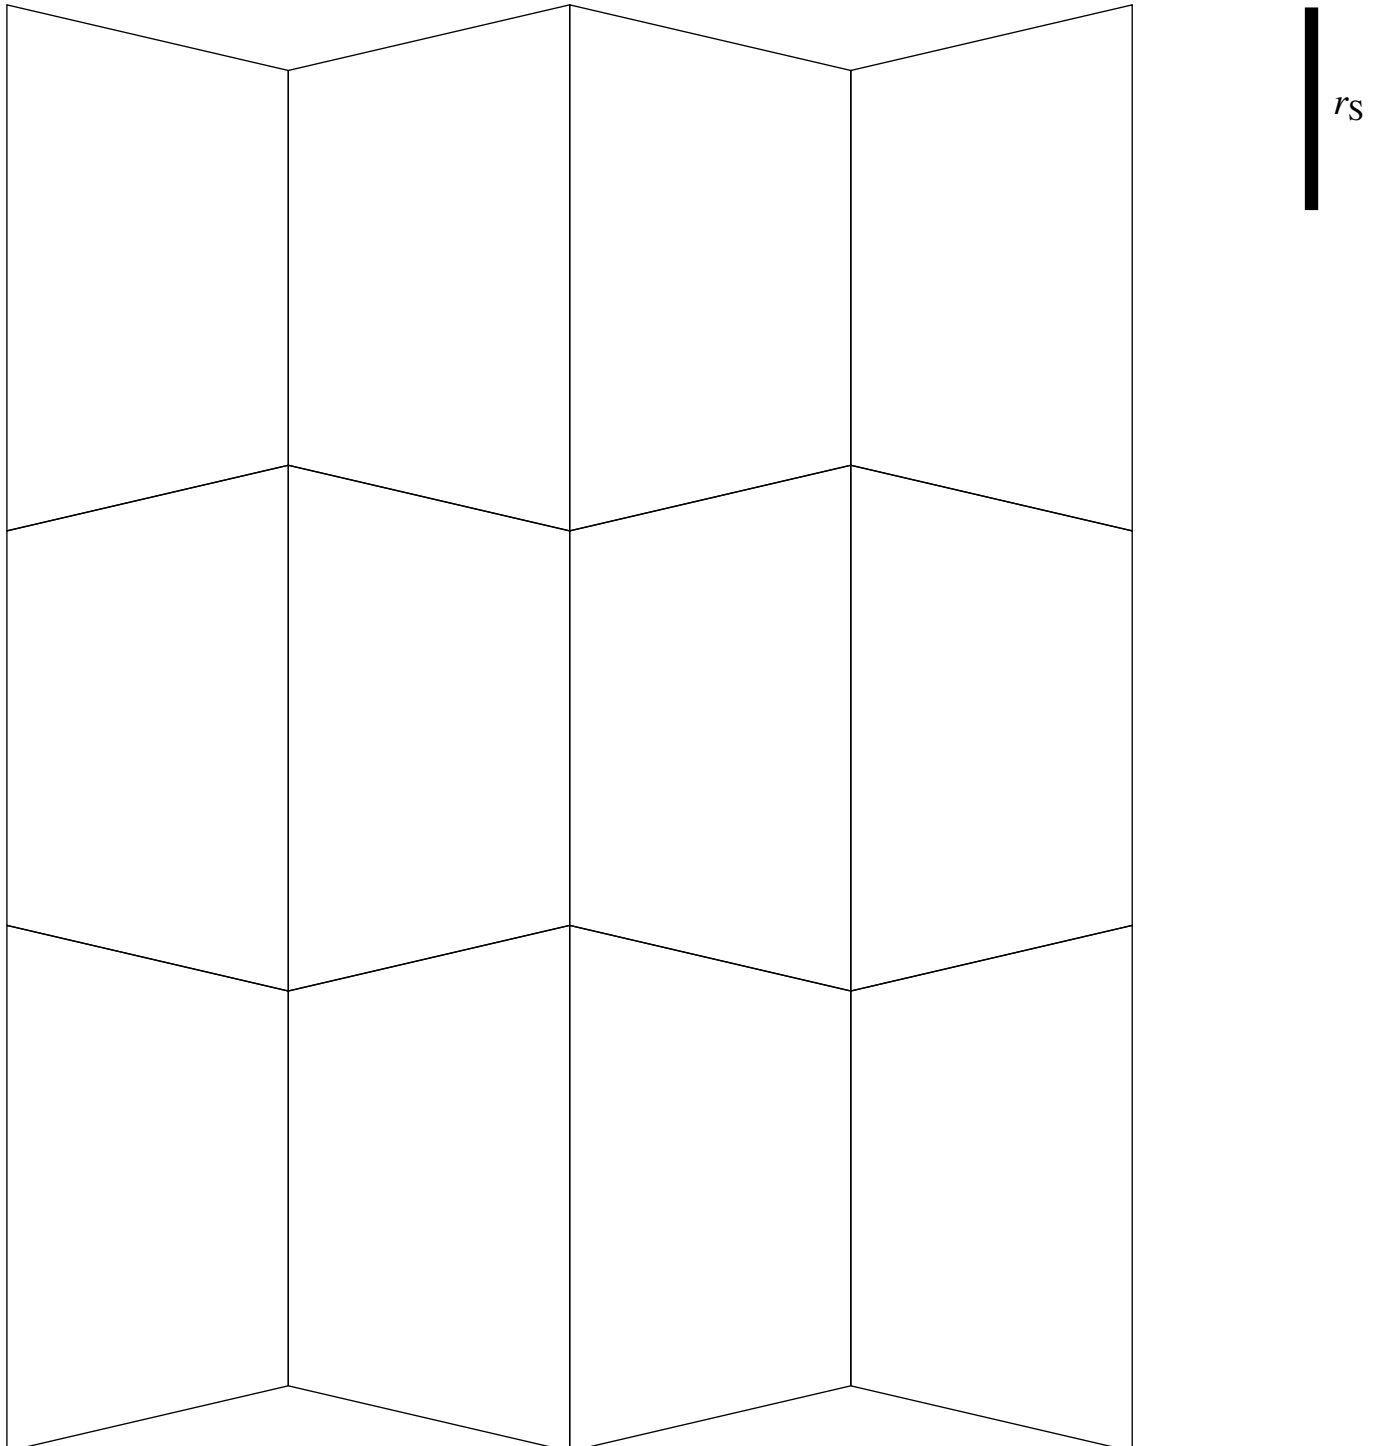

# Sector model of the equatorial plane of a black hole

(enlarge to A3)

Sectors arranged symmetrically, for use with transfer sectors

## Sektormodell der Äquatorfläche eines Schwarzen Lochs

(auf A3 vergrößern)

Sektoren in symmetrischer Anordnung, zur Verwendung mit Transfersektoren

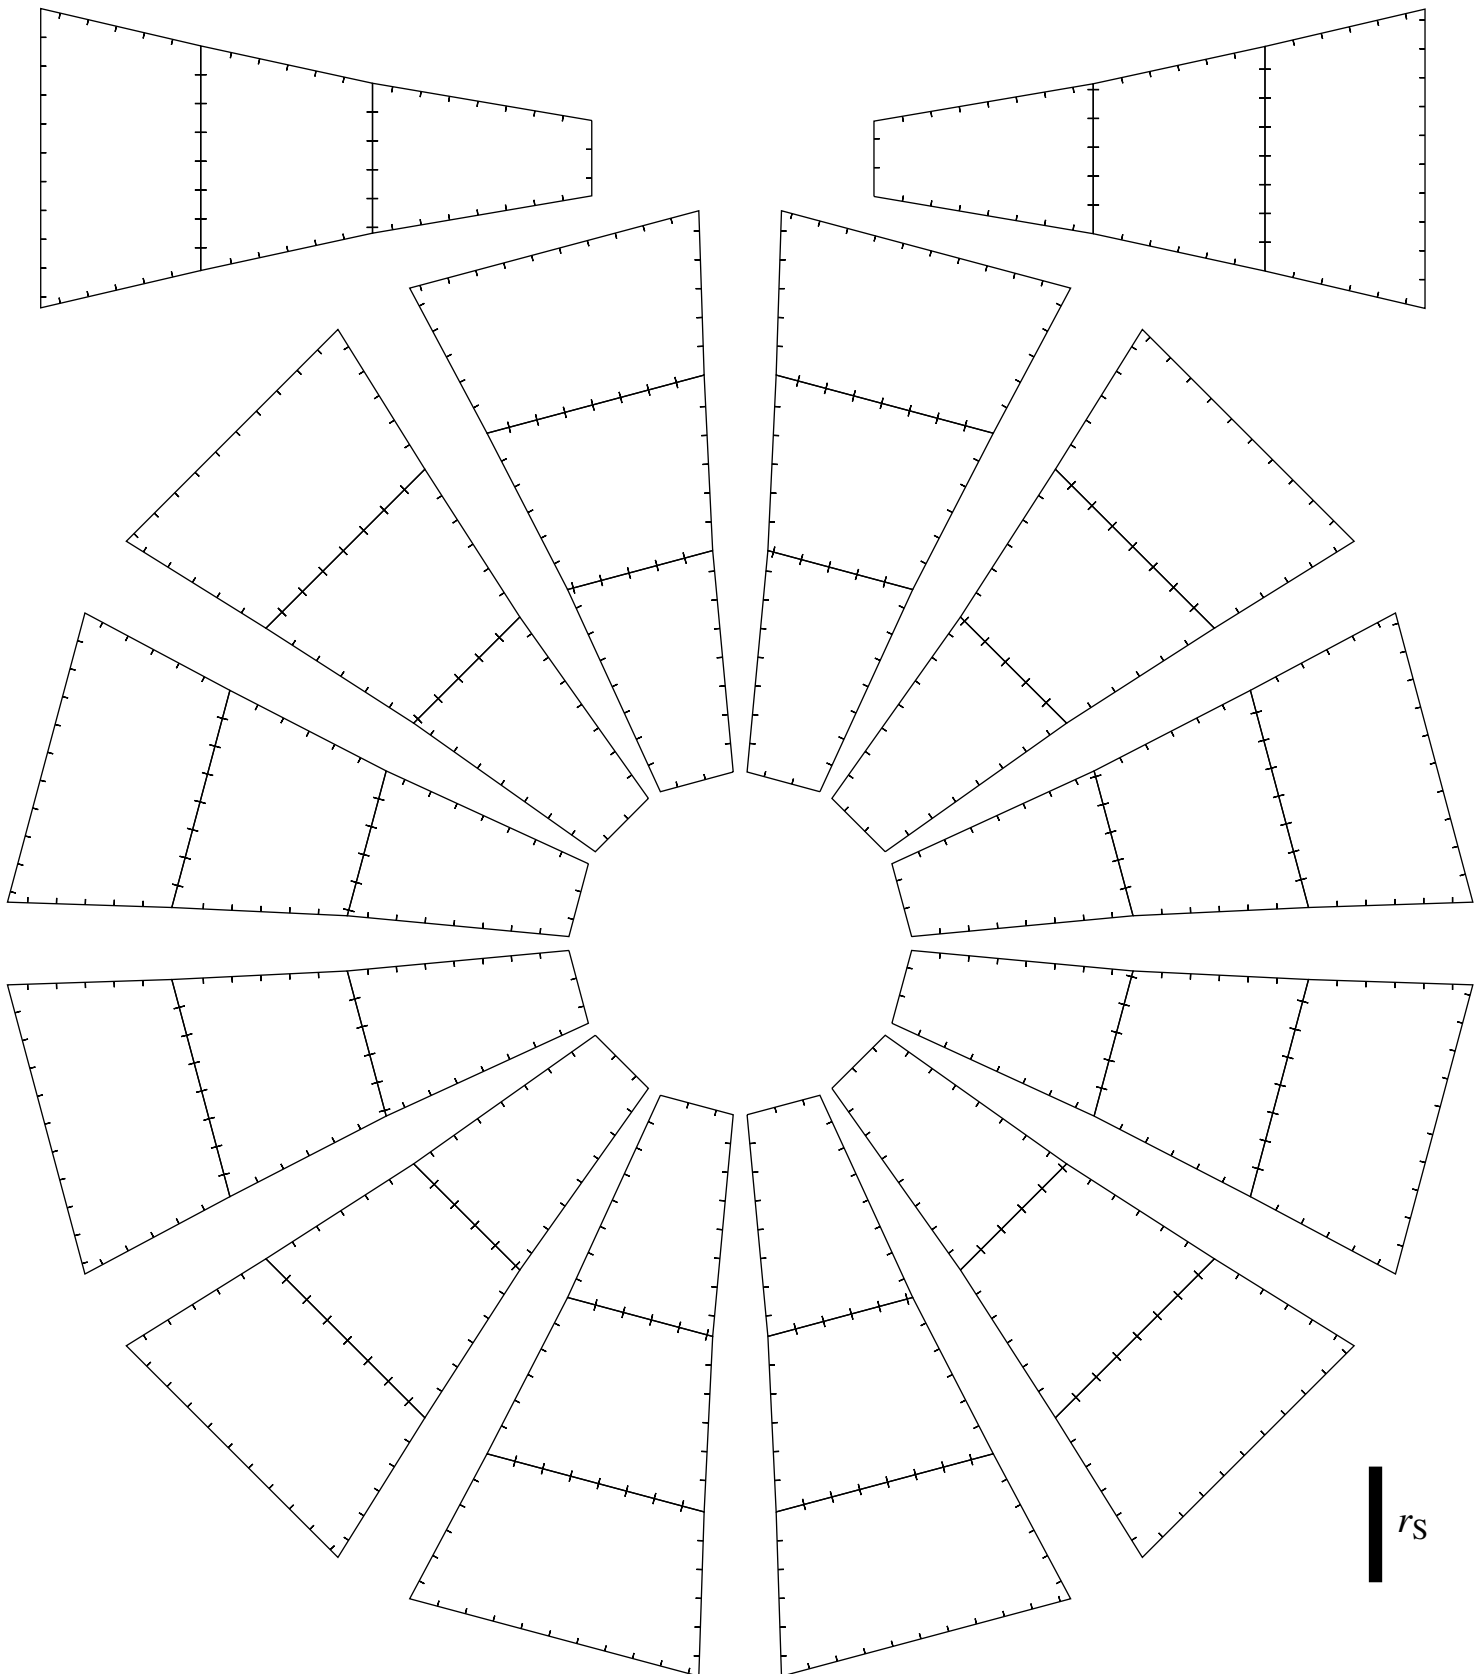

# Sector model of the equatorial plane of a black hole

(enlarge to A3)

Sectors arranged symmetrically, for use with transfer sectors

With marking for a single geodesic

## Sektormodell der Äquatorfläche eines Schwarzen Lochs

(auf A3 vergrößern)

Sektoren in symmetrischer Anordnung, zur Verwendung mit Transfersektoren

Mit Startstrich für eine Geodäte

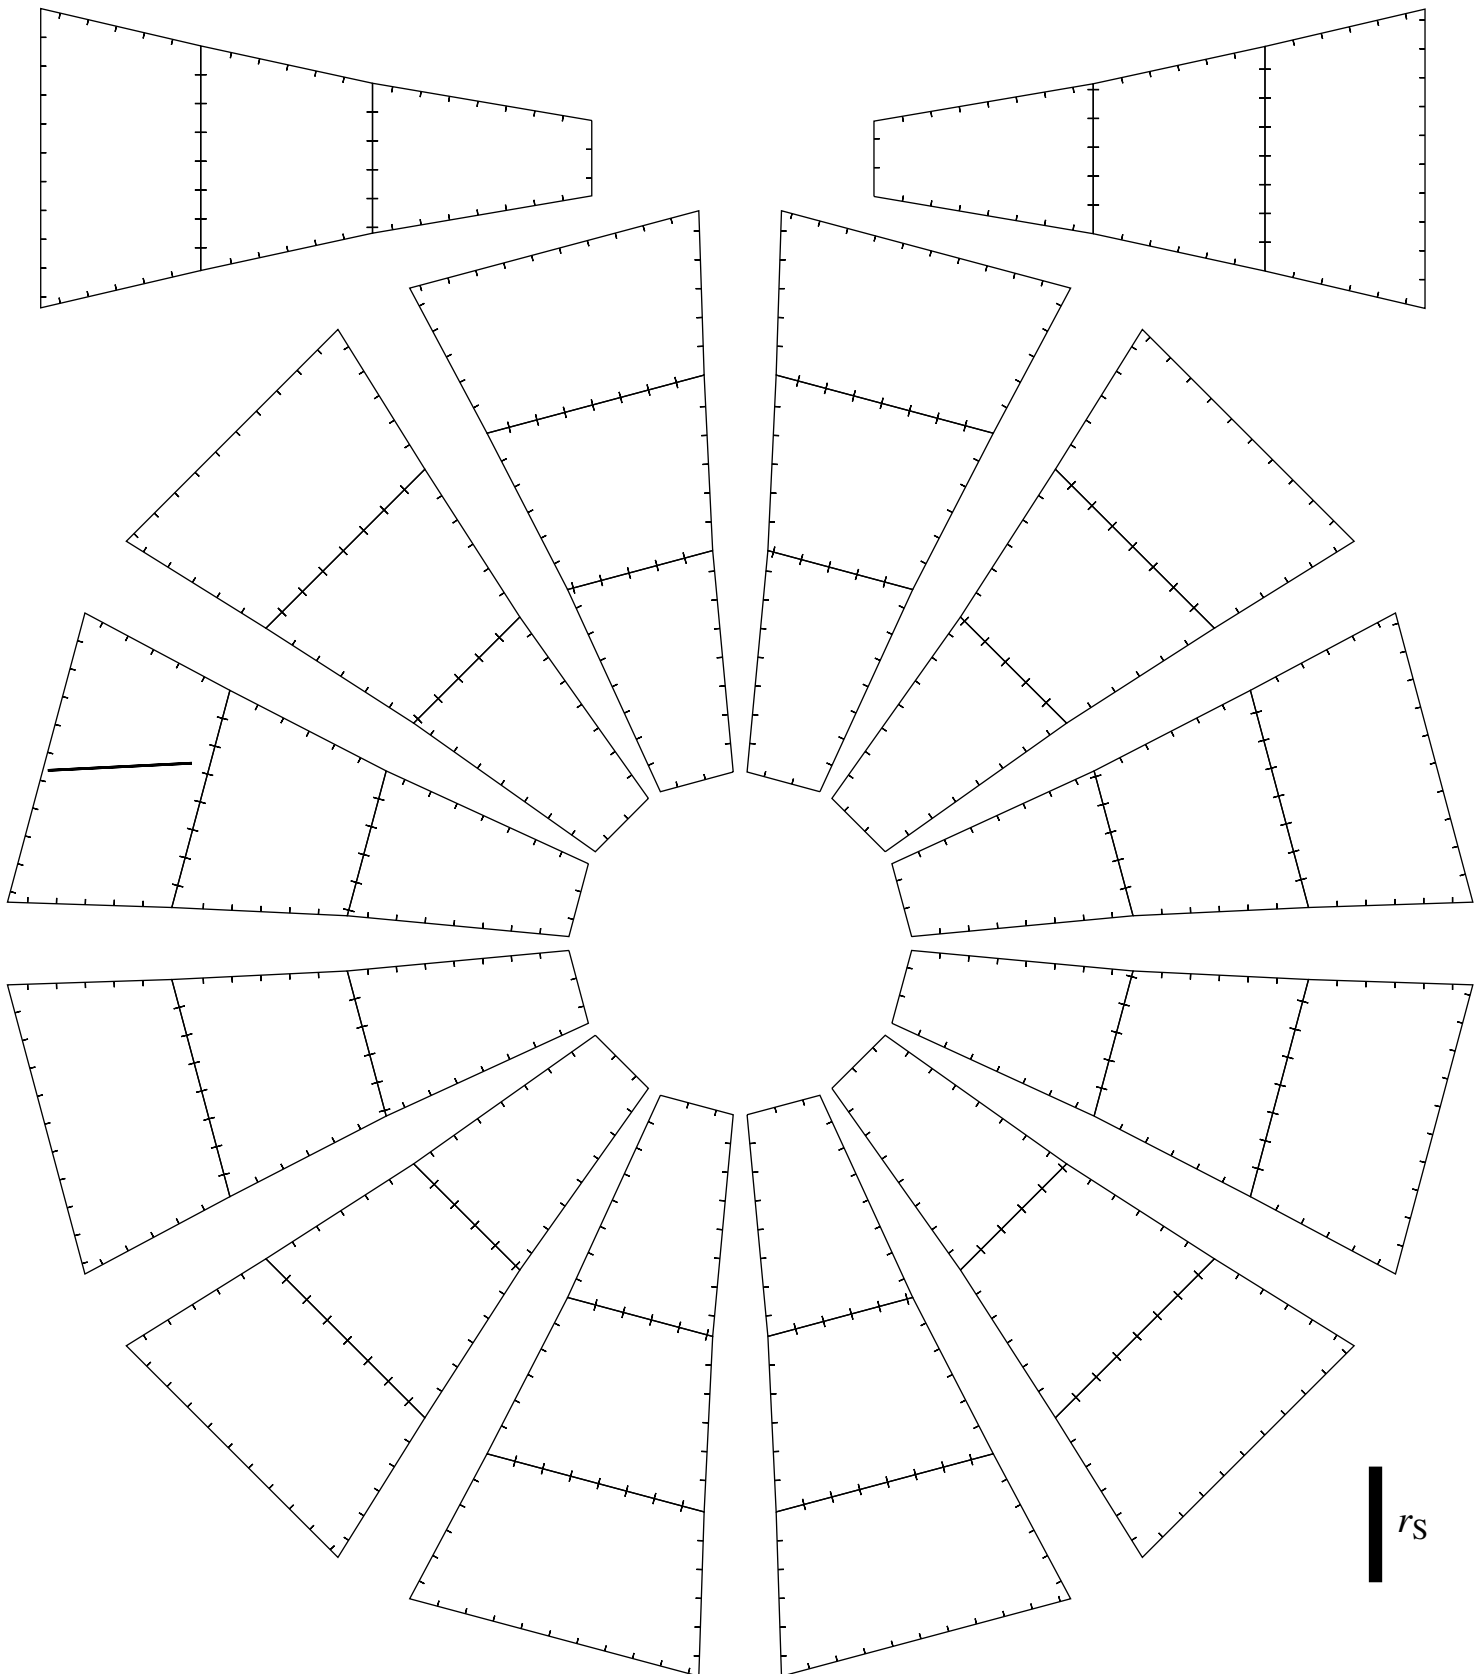

(enlarge to A3)

Sectors arranged symmetrically, for use with transfer sectors

With markings for two geodesics forming a digon

# Sektormodell der Äquatorfläche eines Schwarzen Lochs (auf A3 vergrößern)

## Sektoren in symmetrischer Anordnung, zur Verwendung mit Transfersektoren

Mit Startstrichen für zwei Geodäten, die ein Zweieck bilden

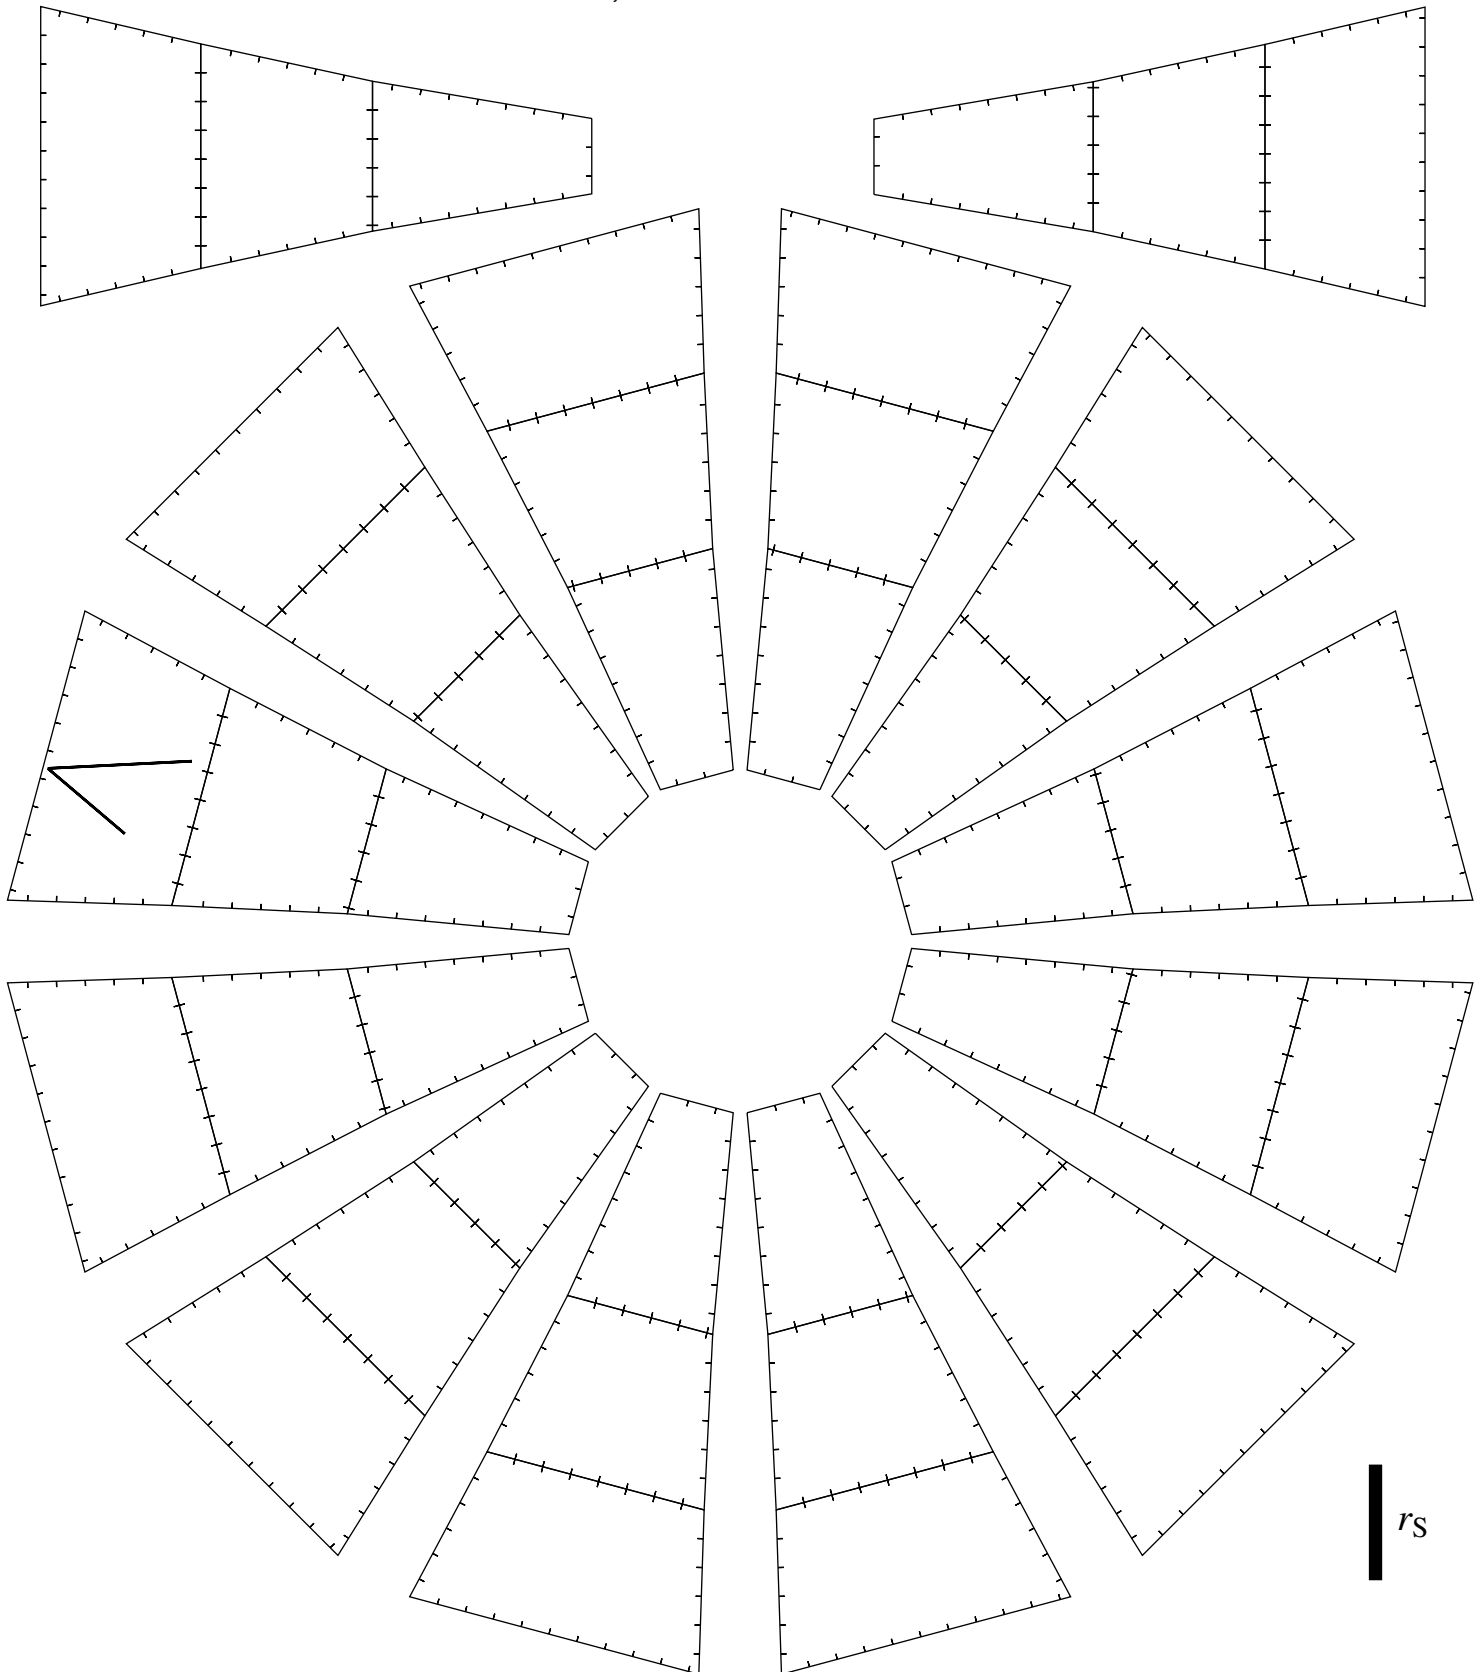



# Sector model of the equatorial plane of a black hole

(enlarge to A3)

Sectors arranged symmetrically, for use with transfer sectors

With markings for two initially parallel geodesics

## Sektormodell der Äquatorfläche eines Schwarzen Lochs

(auf A3 vergrößern)

Sektoren in symmetrischer Anordnung, zur Verwendung mit Transfersektoren

Mit Startstrichen für zwei parallel startende Geodäten

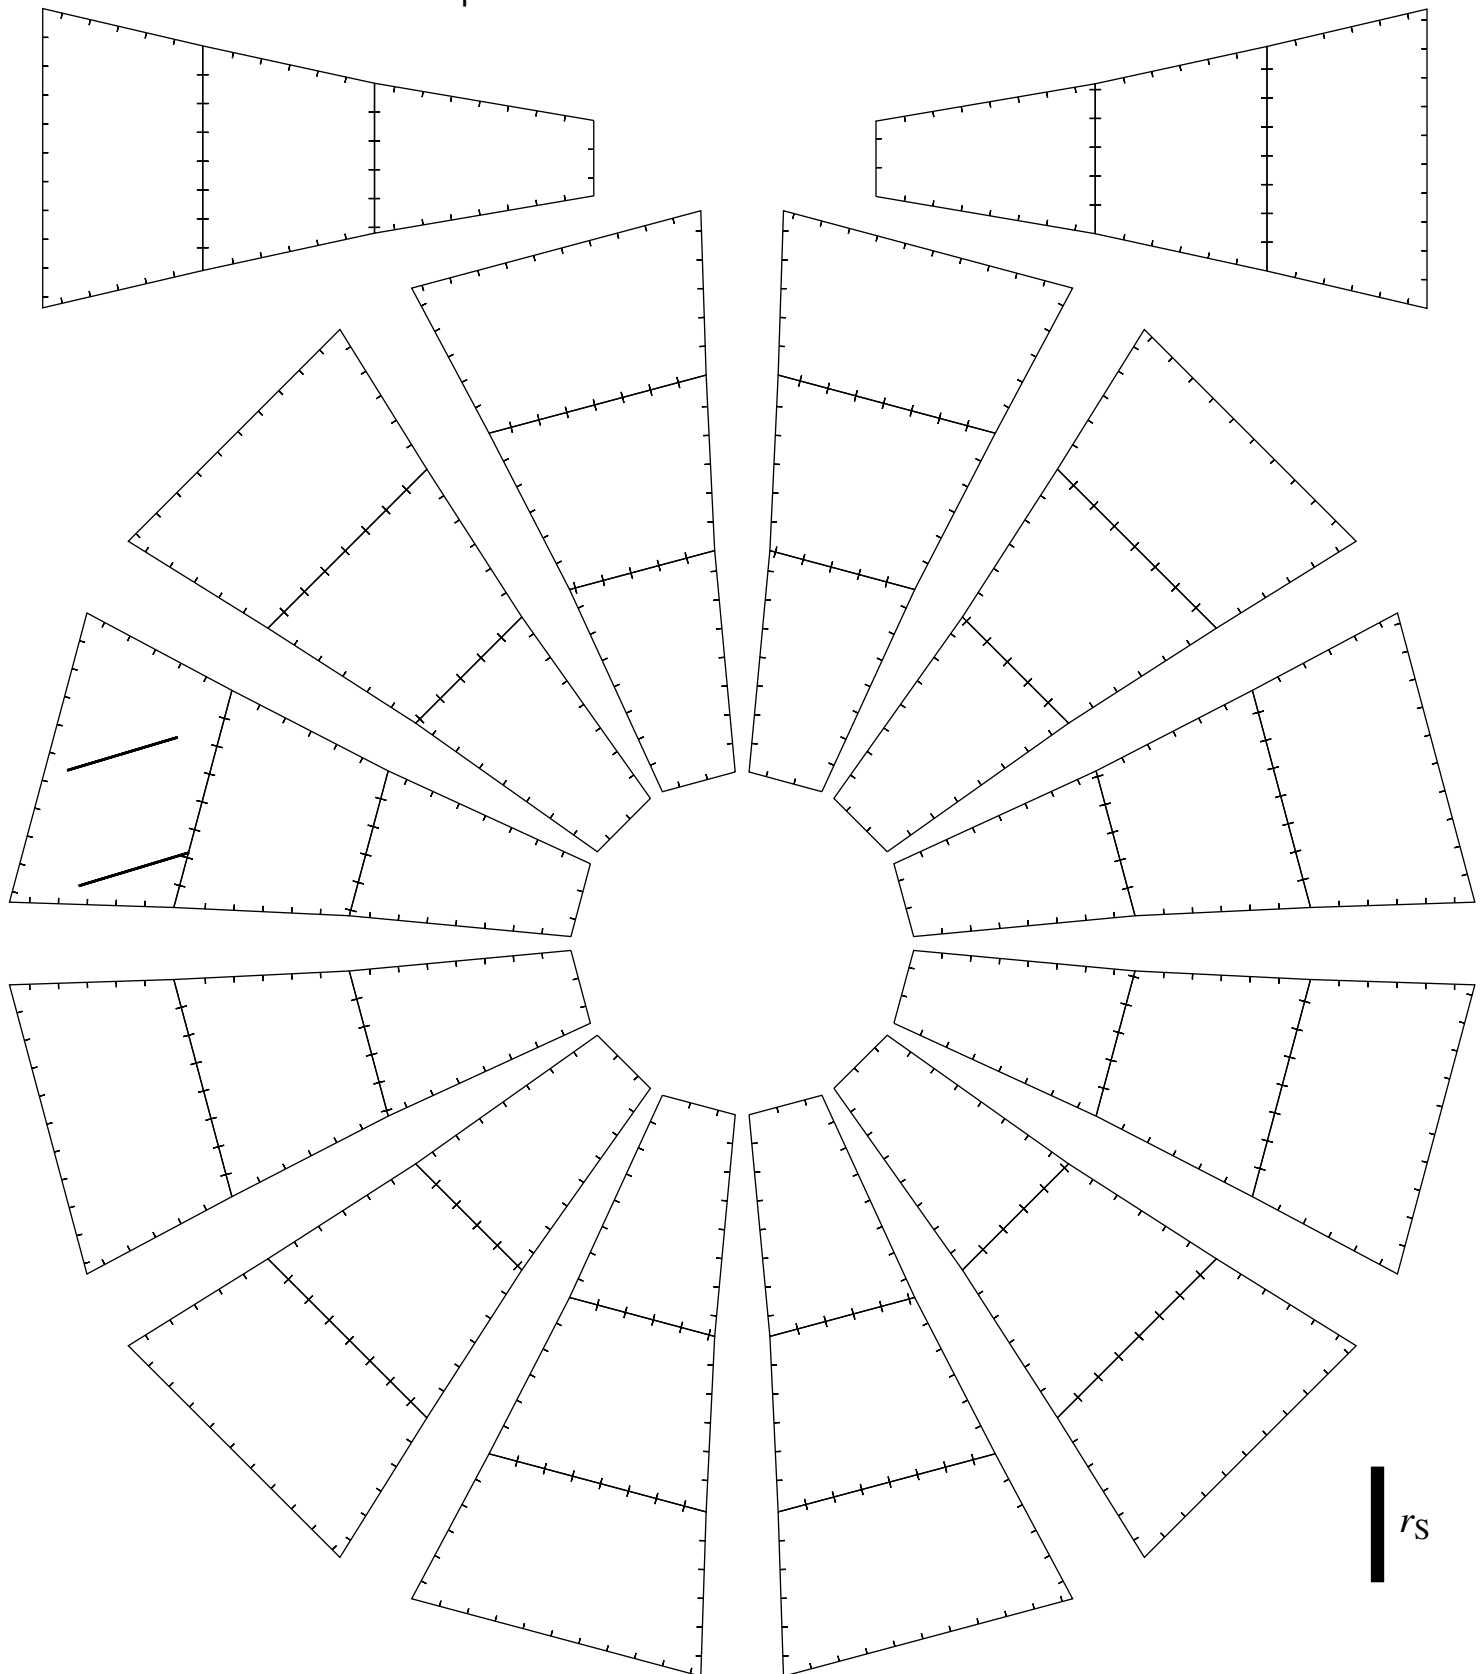

# Sector model of the equatorial plane of a black hole

With a single geodesic

## Sektormodell der Äquatorfläche eines Schwarzen Lochs

Mit einer Geodäten

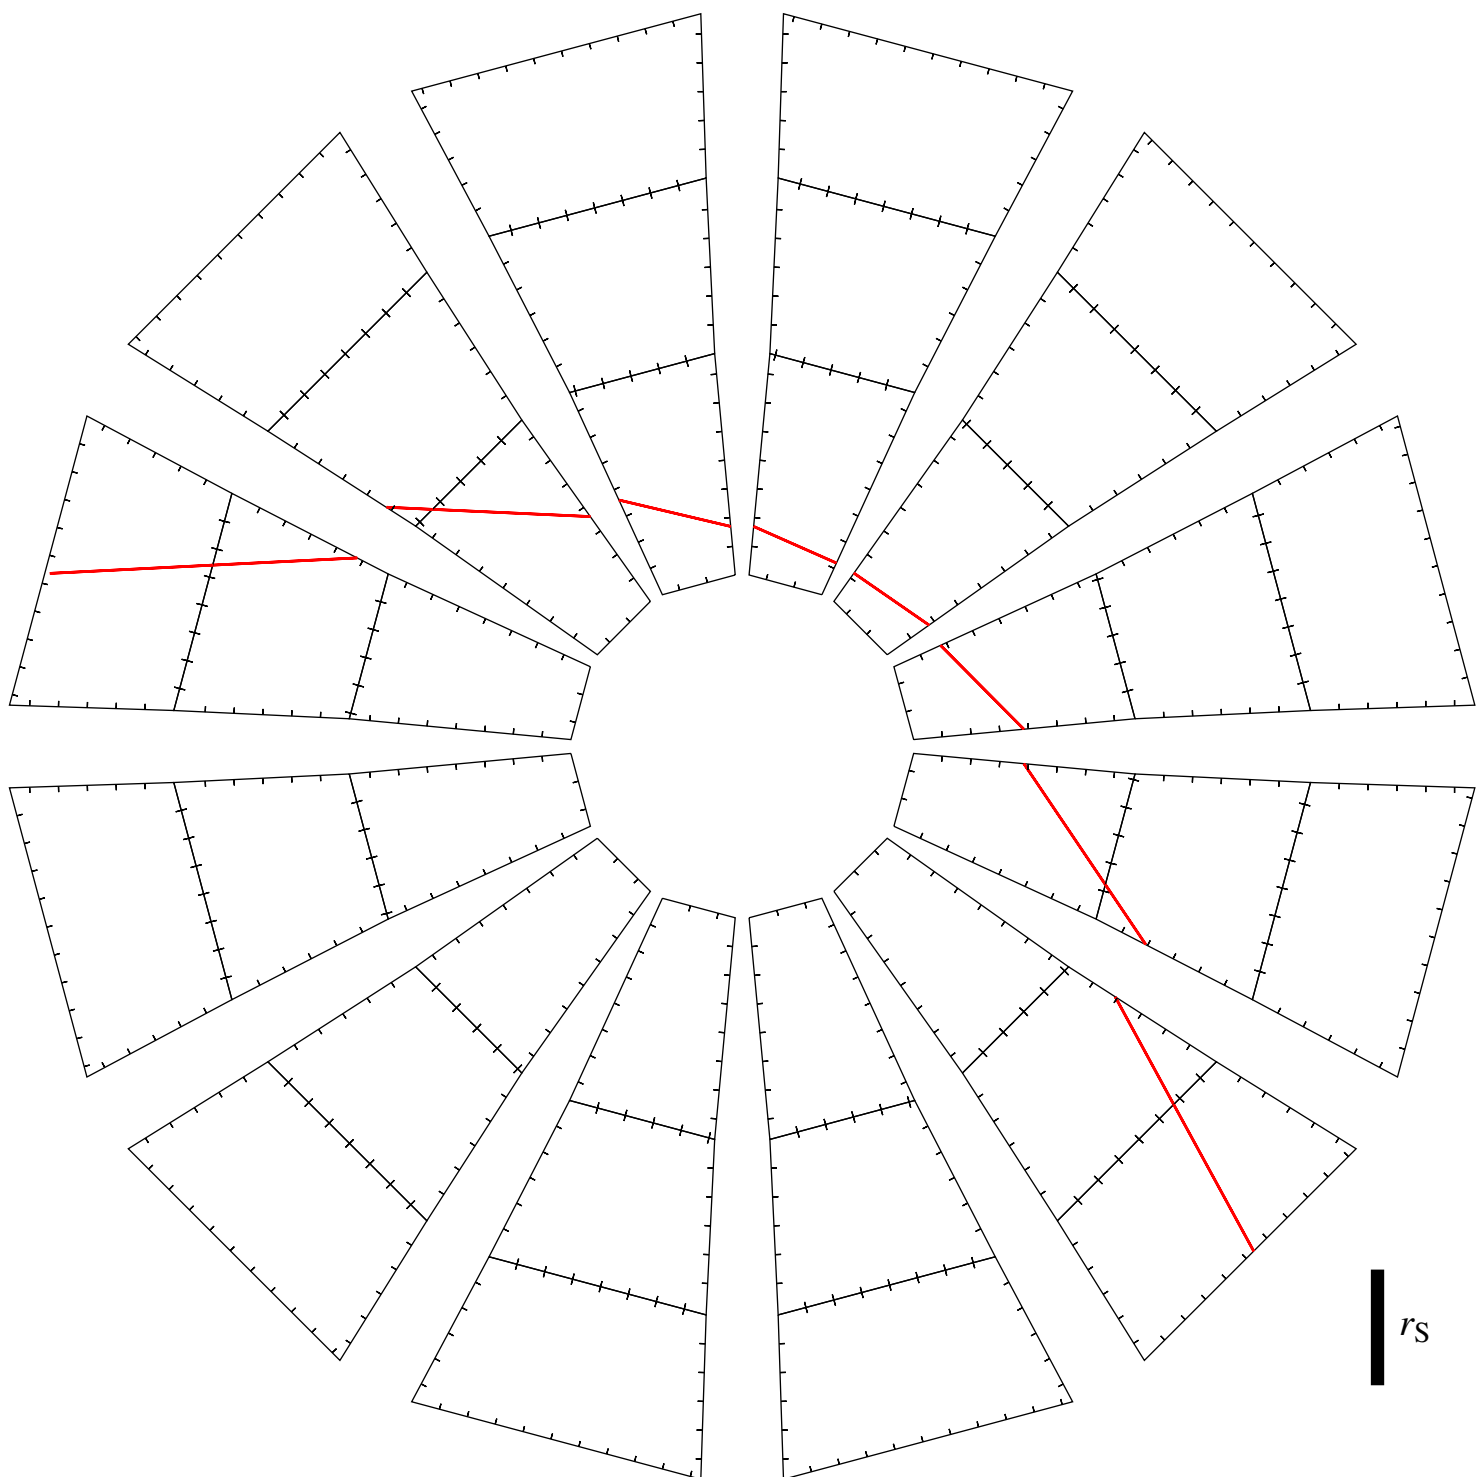

# Sector model of the equatorial plane of a black hole

With two geodesics forming a digon

## Sektormodell der Äquatorfläche eines Schwarzen Lochs

Mit zwei Geodäten, die ein Zweieck bilden

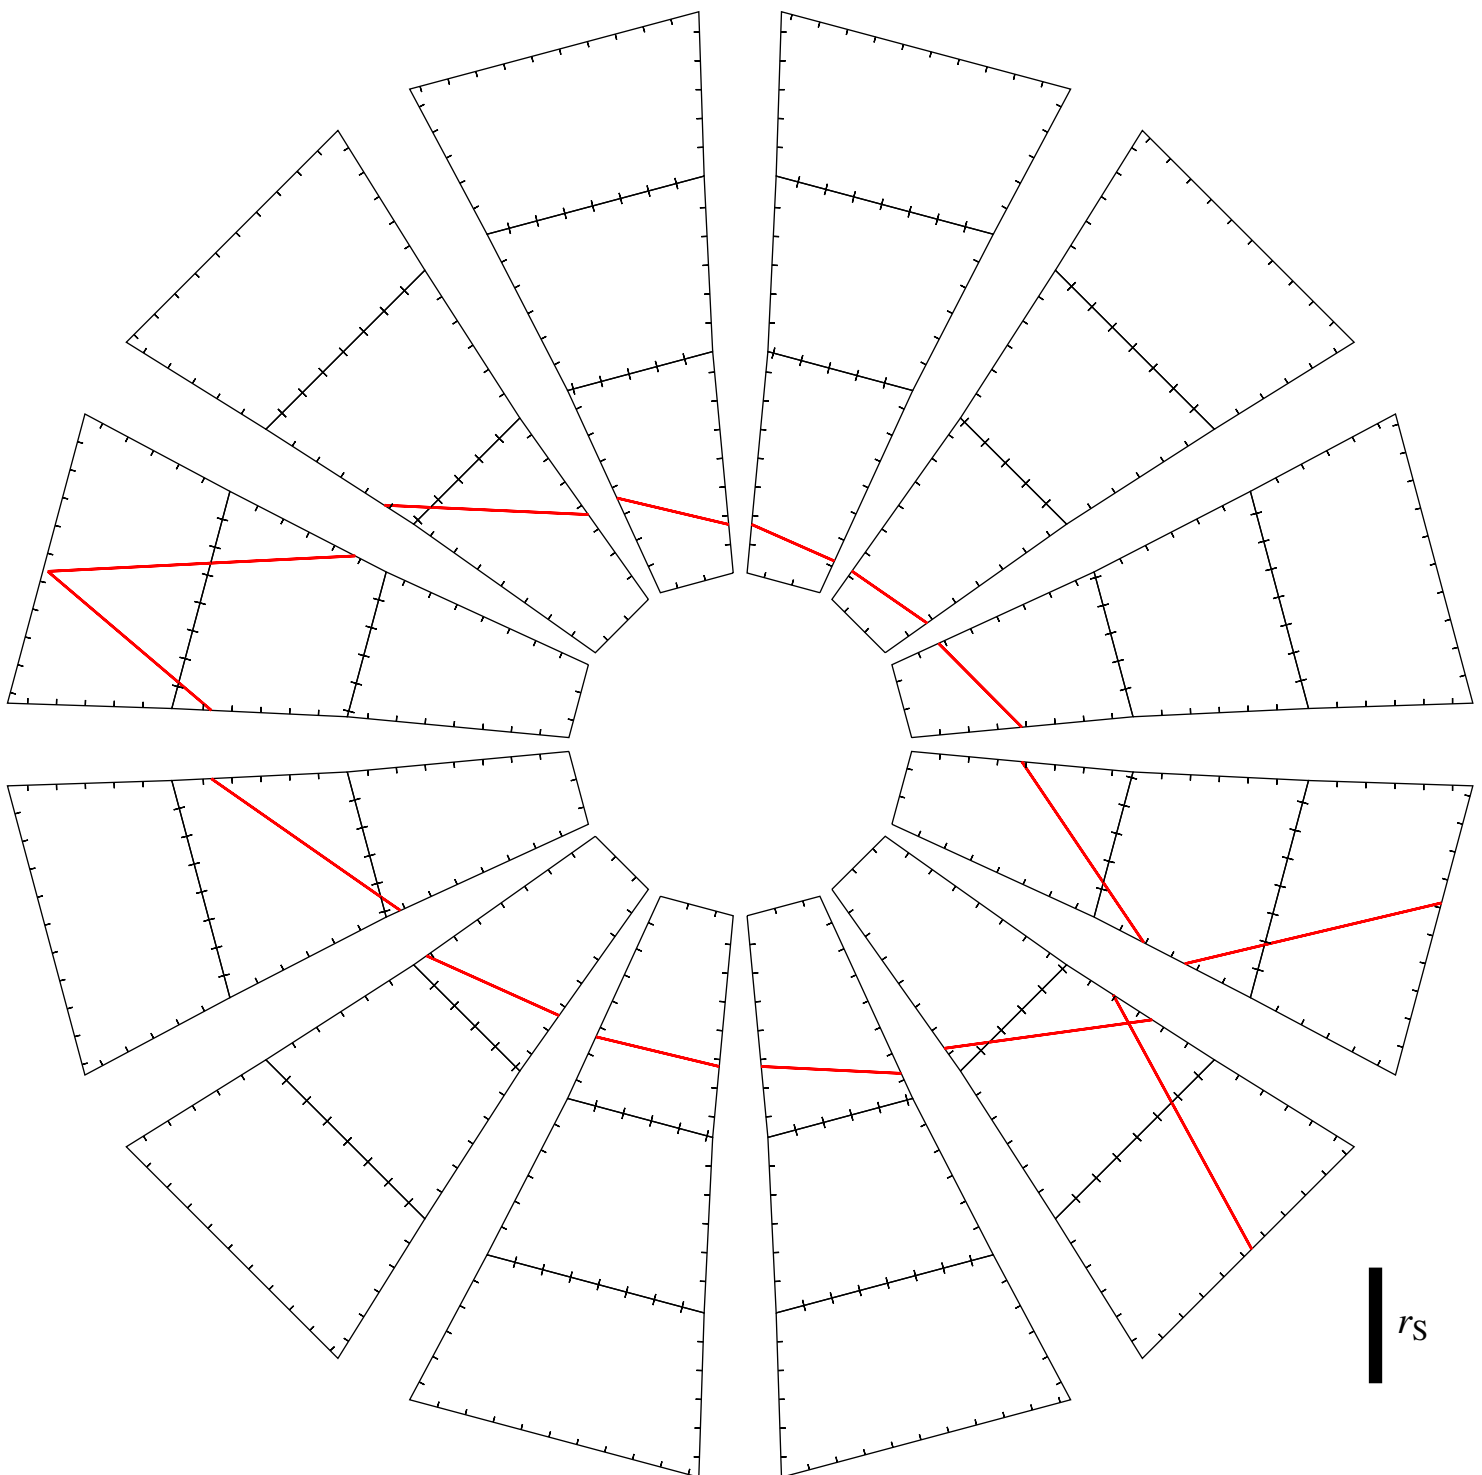

# Sector model of the equatorial plane of a black hole

With two initially parallel geodesics

## Sektormodell der Äquatorfläche eines Schwarzen Lochs

Mit zwei parallel startenden Geodäten

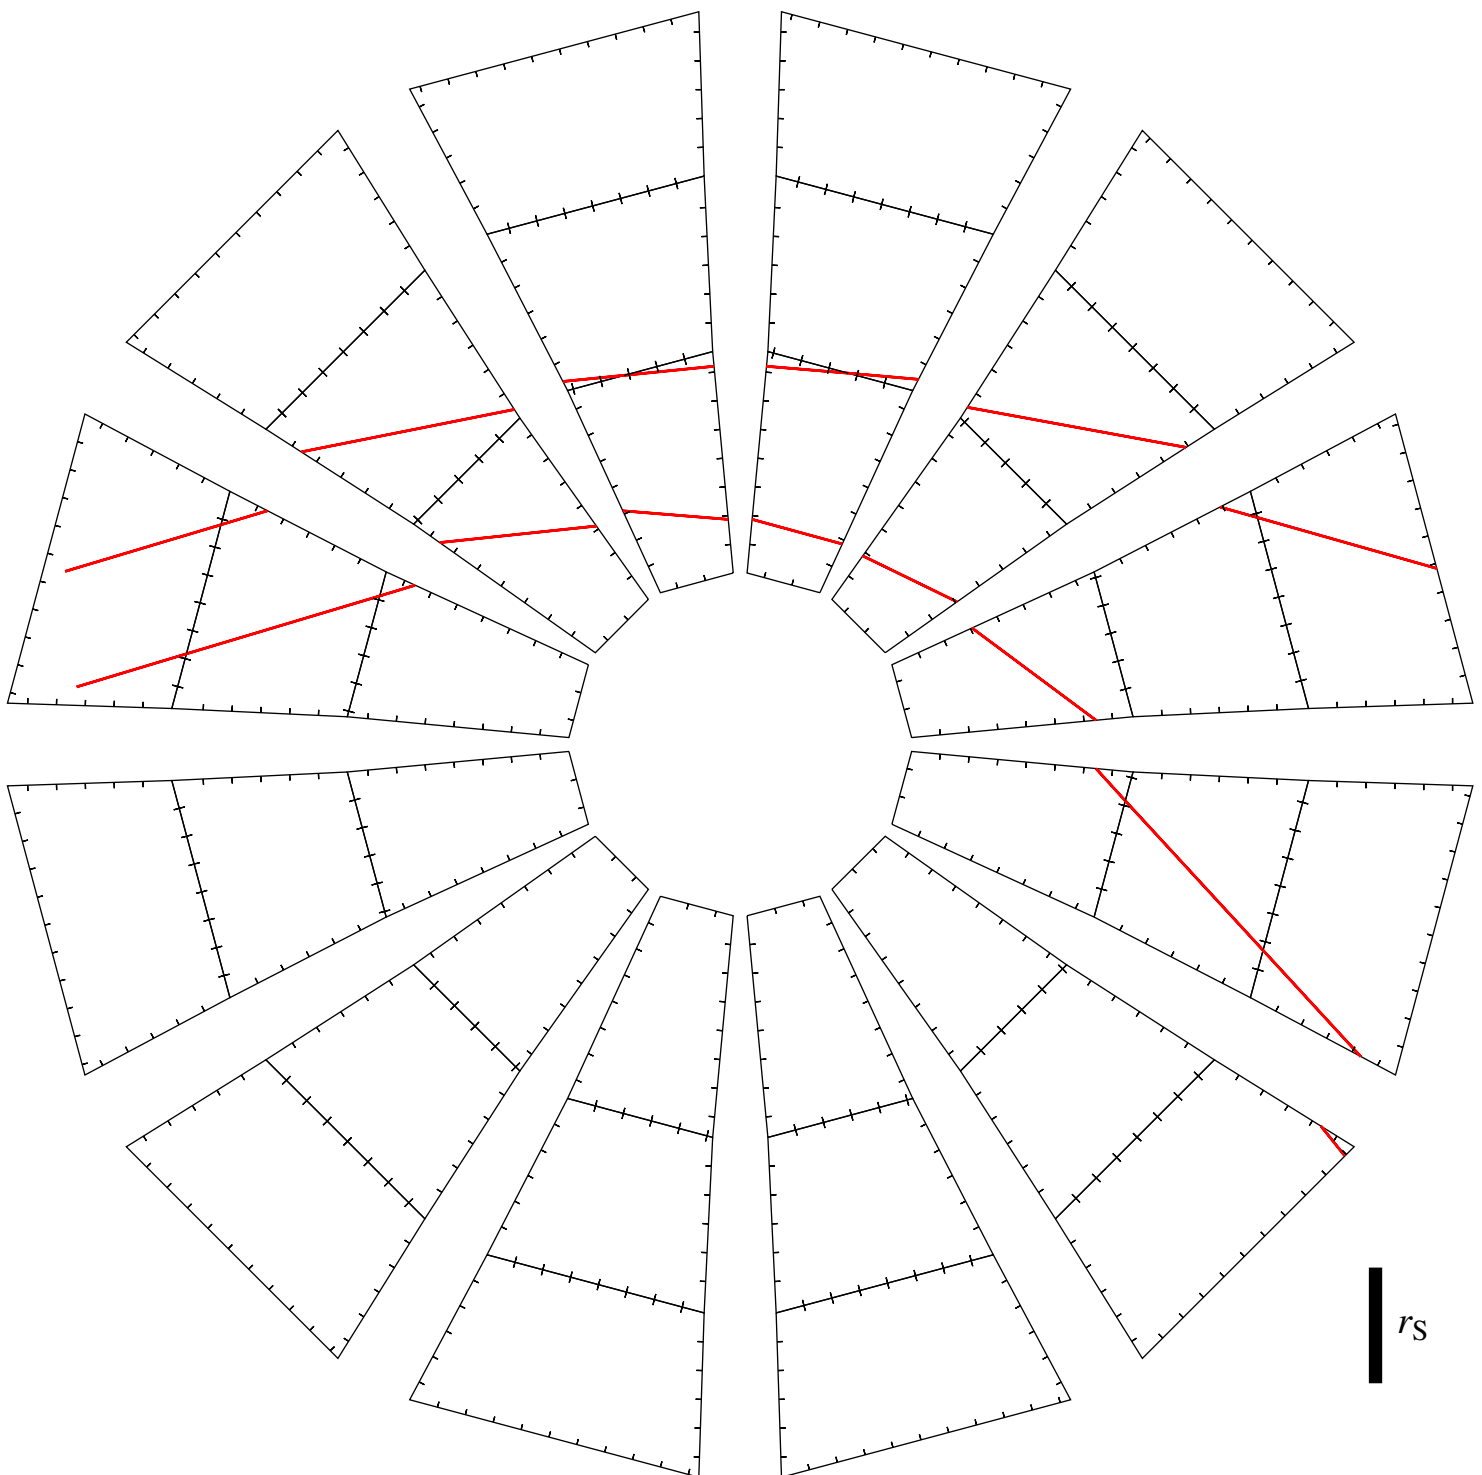

Supplement: Supplementary file 1 [file worksheets2.pdf]
